# Supplementary material for: Lotto: Secure Participant Selection against Adversarial Servers in Federated Learning
Source: arXiv:2401.02880 source file (2024-03-06)
Supplement: Supplementary file 1 [file complexity.tex]

%!TEX root = ../main.tex
\section{Complexity Analysis}
~\label{sec:appendix_complexity}

Let $n$ be the initial population size, and $s$ the target number of sampled clients. We also abuse the symbol $n$ to represent the refined population size, as both should be of the same magnitude.
For secure random selection, \texttt{Client-Centric} induces an overhead of $O(1)$ and $O(n + s^2)$ to the server's computation and communication, respectively, while those incurred to a selected client are $O(s)$ and $O(s)$, respectively.
In \texttt{Server-Centric}, the computation and communication for the server are $O(n)$ and $O(s^2)$, respectively, while those for a selected client are $O(s)$ and $O(s)$, respectively.
For informed selection, the overhead of the server's computation in \texttt{Client-Centric} becomes $O(n)$, while other terms of overhead remain the same, compared to random selection.
