# Supplementary material for: Lotto: Secure Participant Selection against Adversarial Servers in Federated Learning
Source: arXiv:2401.02880 source file (2024-03-06)
Supplement: Supplementary file 2 [file selection.tex]

%!TEX root = ../main.tex
\section{Effectiveness of Over-Selection}
~\label{sec:appendix_overselection}

In \system{}, a fixed sample size is achieved via over-selection with residual removal (\cref{sec:design_random}).
The theorem below captures the relationship between the over-selection factor $\alpha$ and the success rate of selecting enough participants in one go.

\begin{theorem}[Effectiveness of Over-Selection]
	Using an over-selection factor $\alpha>0$, the described process in \system{} results in at least $s$ candidates with probability of $1 - \sum_{i = 0}^{\lfloor s - 1 \rfloor} \binom{n_{true}}{i} p^i (1-p)^{n_{true} - i}$ where $p = \alpha s /n_{true}$ and $n_{true}$ is the actual size of the population.
	\label{thm:over_selection}
\end{theorem}

%The proof is trivial and thus omitted for brevity.
